# Supplementary material for: NetScatter: Enabling Large-Scale Backscatter Networks
Source: arXiv:1808.05195 source file (2018-08-15)
Supplement: Supplementary file 1 [file appendix.tex]

\begin{figure}[t]
	\begin{subfigure}{\columnwidth}
    	\centering
    	\includegraphics[width=1\linewidth]{./figs/15_appendix/1_no_padding_no_fraction_time.eps}
		\label{testXX}
        \vskip -0.2in
        \caption{}
	\end{subfigure}
    \vskip -0.05in
    \begin{subfigure}{\columnwidth}
    	\centering
    	\includegraphics[width=1\linewidth]{./figs/15_appendix/1_no_padding_no_fraction_fft.eps}
		\label{fig:no_padding_no_fraction_fft}
        \vskip -0.2in
        \caption{}
	\end{subfigure}
    \begin{subfigure}{\columnwidth}
    	\centering
    	\includegraphics[width=1\linewidth]{./figs/15_appendix/2_padding_no_fraction_time.eps}
		\label{fig:padding_no_fraction_time}
        \vskip -0.2in
        \caption{}
	\end{subfigure}
    \vskip -0.05in
    \begin{subfigure}{\columnwidth}
    	\centering
    	\includegraphics[width=1\linewidth]{./figs/15_appendix/2_padding_no_fraction_fft.eps}
		\label{fig:padding_no_fraction_fft}
        \vskip -0.2in
        \caption{}
	\end{subfigure}
    \vskip -0.05in
    \begin{subfigure}{\columnwidth}
    	\centering
    	\includegraphics[width=1\linewidth]{./figs/15_appendix/3_no_padding_fraction_fft.eps}
		\label{fig:no_padding_fraction_fft}
        \vskip -0.2in
        \caption{}
	\end{subfigure}
    \vskip -0.05in
    \begin{subfigure}{\columnwidth}
    	\centering
    	\includegraphics[width=1\linewidth]{./figs/15_appendix/4_padding_fraction_fft.eps}
		\label{fig:padding_fraction_fft}
        \vskip -0.2in
        \caption{}
	\end{subfigure}
	\vskip -0.1in
\caption{{\bf Zero-padding explanation.} Discrete Time and FFT domain results of different cases of signal with and without zero-padding.}
	\label{fig:zeropad}
    \vskip -0.15in
\end{figure}

\section{Zero-padding and FFT Resolution}\label{sec:appendix}
In this appendix, we prove that zero-padding will increase the resolution of finding FFT peaks in CSS demodulation process. Although the theory holds for all cases, we will prove it in the context of CSS modulation. Assume we are sending an upchirp which result in a peak in the $k^{th}$ FFT bin. After multiplying by downchirp, we would have $x[n]$ in discrete time domain and equal to\footnote{Small letters are used for discrete time domain signal representations and capital for discrete FFT domain.}:
\begin{equation*}
x[n]=A~exp(j2\pi\frac{k}{2^{SF}}n)
\end{equation*}
In which, $A$ is the amplitude of the demodulated signal. Fig.~\ref{fig:zeropad}(a) shows the continuous time domain signal, $Real\{x(t)\}$, and its sampled discrete time signal $Real\{x[n]\}$ with $SF=4$, $k=3$ and $A=1$. Assuming sampling rate is equal to $BW=500~KHz$. The $2^{SF}$-point FFT of $x[n]$ would be (Fig.~\ref{fig:zeropad}(b)):

\begin{equation*}
X[n]=\mathscr{F}\{x[n]\}=\delta(n-k)
\end{equation*}

Now, we do $\alpha$-times zero-padding for $x[n]$ to get $x_{z}[n]$. Fig.~\ref{fig:zeropad}(c) shows $Real\{x_{z}[n]\}$ in discrete and continuous time-domain with $\alpha=2$. $x_{z}[n]$ is effectively the result of multiplication of a pulse signal, $p[n]$, and $x_{\alpha}[n]$ in which $x_{\alpha}[n]$ is $x(t)$ with $\alpha2^{SF}$ samples and with the same sampling rate as $x[n]$. The following equations hold for discrete time domain and $\alpha2^{SF}$-point FFT of the $X_{z}[n]$.

\begin{equation*}
x_{z}[n]=x_{\alpha}[n]~p[n] 
\end{equation*}

\begin{equation*}
X_{z}[n]=\mathscr{F}\{x_{\alpha}[n]\}\ast\mathscr{F}\{p[n]\}=X_{\alpha}[n]\ast P[n]
\end{equation*}

Since we have $\alpha2^{SF}$ samples in time-domain and do $\alpha2^{SF}$-point FFT with the same sampling rate, the FFT bin resolution is improved from $\frac{BW}{2^{SF}}$ to $\frac{BW}{\alpha2^{SF}}$. Note that this increase in FFT resolution does not come for free. Since $P[n]$ is a sinc function, convolution with $P[n]$ adds side-lobes to the $X_{z}[n]$ (Fig.~\ref{fig:zeropad}(d)). However, the benefit of increasing the FFT resolution using zero-padding manifests itself when there is fractional frequency or timing mismatch. For example assuming $k=3.5$, the $X[n]$ would be like Fig.~\ref{fig:zeropad}(e), which means we cannot distinguish the FFT peak and demodulate the signal. However, with zero-padding the FFT results would be just a cyclic shift of FFT results of previous case with $k=3$, Fig.~\ref{fig:zeropad}(f). As a result, we can improve detection of the FFT peak and demodulation of the signal by doing zero-padding.
